# Supplementary material for: Growth of hexagonal BN crystals by traveling-solvent floating zone
Source: arXiv:2412.17195 ancillary file (2025-04-08)
Supplement: Supplementary file 1 [file SupplementaryInformation.pdf]

**Supplemental Information for "Growth of hexagonal BN by traveling-solvent floating zone"**

Eli Zoghlin[a*], Juliette Plo[b] , Gaihua Ye[c], Cynthia Nnokwe[c], Reina Gomez[d], Austin Ferrenti[e], Satya Kushwaha[a,e], Rui He[c], Stephen D. Wilson[d], Guillaume Cassabois[b,f], James H. Edgar[g], Tyrel M. McQueen[a,e,h,**]

a) William H. Miller III Department of Physics and Astronomy, The Johns Hopkins University, Baltimore, Maryland 21218, United States
b) Laboratoire Charles Coulomb, Université de Montpellier and CNRS, Montpellier 34095, France
c) Department of Electrical and Computer Engineering, Texas Tech University, Lubbock, Texas 79409, United States
d) Materials Department, University of California Santa Barbara, Santa Barbara, California 93106, United States
e) Department of Chemistry, The Johns Hopkins University, Baltimore, Maryland 21218, United States
f) Institut Universitaire de France, Paris 75231, France
g) Tim Taylor Department of Chemical Engineering, Kansas State University, Manhattan, Kansas 66506, United States
h) Department of Materials Science and Engineering, The Johns Hopkins University, Baltimore, Maryland 21218, United States

*ezoghli1@jh.edu
**mcqueen@jhu.edu

## 1. Optical images and microCT data for additional samples

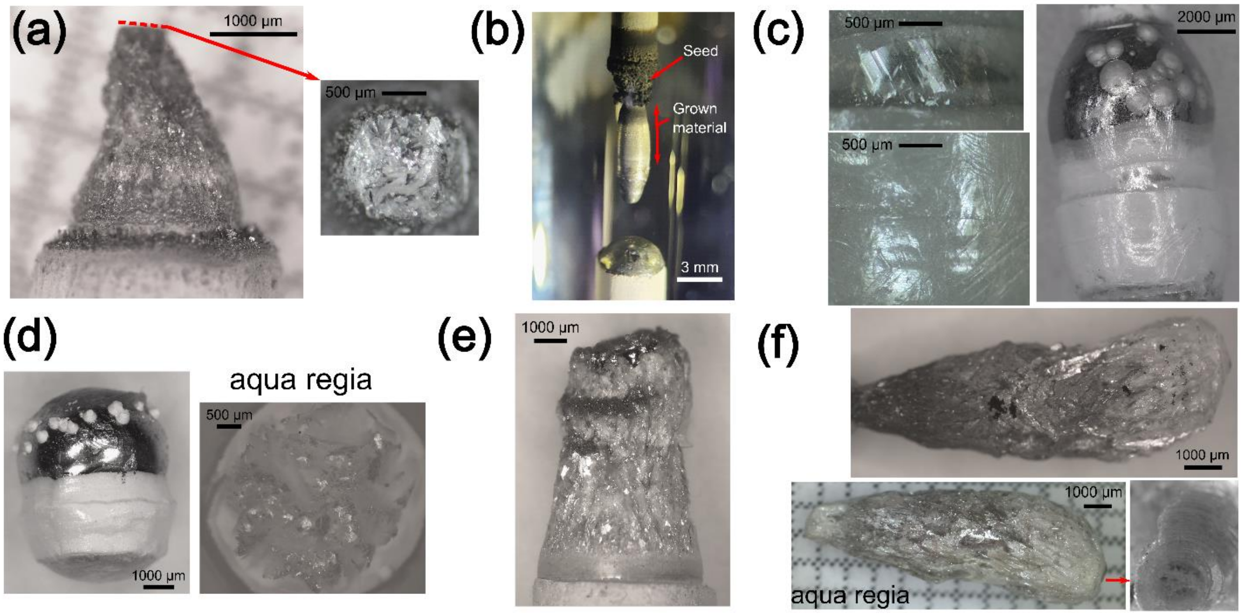


**Figure S1:** Optical images of additional growths conducted in the course of this work. The growth conditions for each sample are provided in the caption. **(a)** FeCr flux, $P$ = 5 bar, 0.1 mm/h, h-BN feed, TSFZ, $\phi$ = 2°, $D_U$ = $D_L$ = 3 mm. This growth is analogous to that shown in Fig. 2c in the main text, but without pre-saturation of the flux with B. **(b)** $FeCrB_{0.2}$ flux, $P$ = 7 bar, 0.1 mm/h, h-BN feed, LPG, $\phi$ = 0°, $D_L$ = 6 mm. The growth was seeded using Stage 1 of the sample shown in Fig. 2c. The image shows the sample still mounted in the furnace at the completion of the growth. **(c)** Fe flux, $P$ = 7 bar, 0.1 mm/h, B feed, TSFZ, $\phi$ = 0°, $D_U$ = 2 – 3 mm, $D_L$ = 6 mm. **(d)** $FeB_{0.2}$ flux, $P$ = 7 bar, 0.1/mm/h, B Feed, TSFZ, $\phi$ = 0°, $D_U$ = 2 mm, $D_L$ = 6 mm. **(e)** $FeCrB_{0.2}$ flux, $P$ = 7 bar, 0.1 mm/h, B feed, TSFZ, $\phi$ = 0°, $D_U$ = 5 mm, $D_L$ = 6 mm. **(f)** $FeCrB_{0.2}$ flux, $P$ = 7 bar, 0.1 mm/h, B feed, LPG, $\phi$ = 0°, $D_U$ = 1 mm, $D_L$ = 6 mm. We note that for the growths shown in **(c)** and **(d)** the recrystallized material is primarily polycrystalline, with crystalline flakes also forming (see Fig. S6).

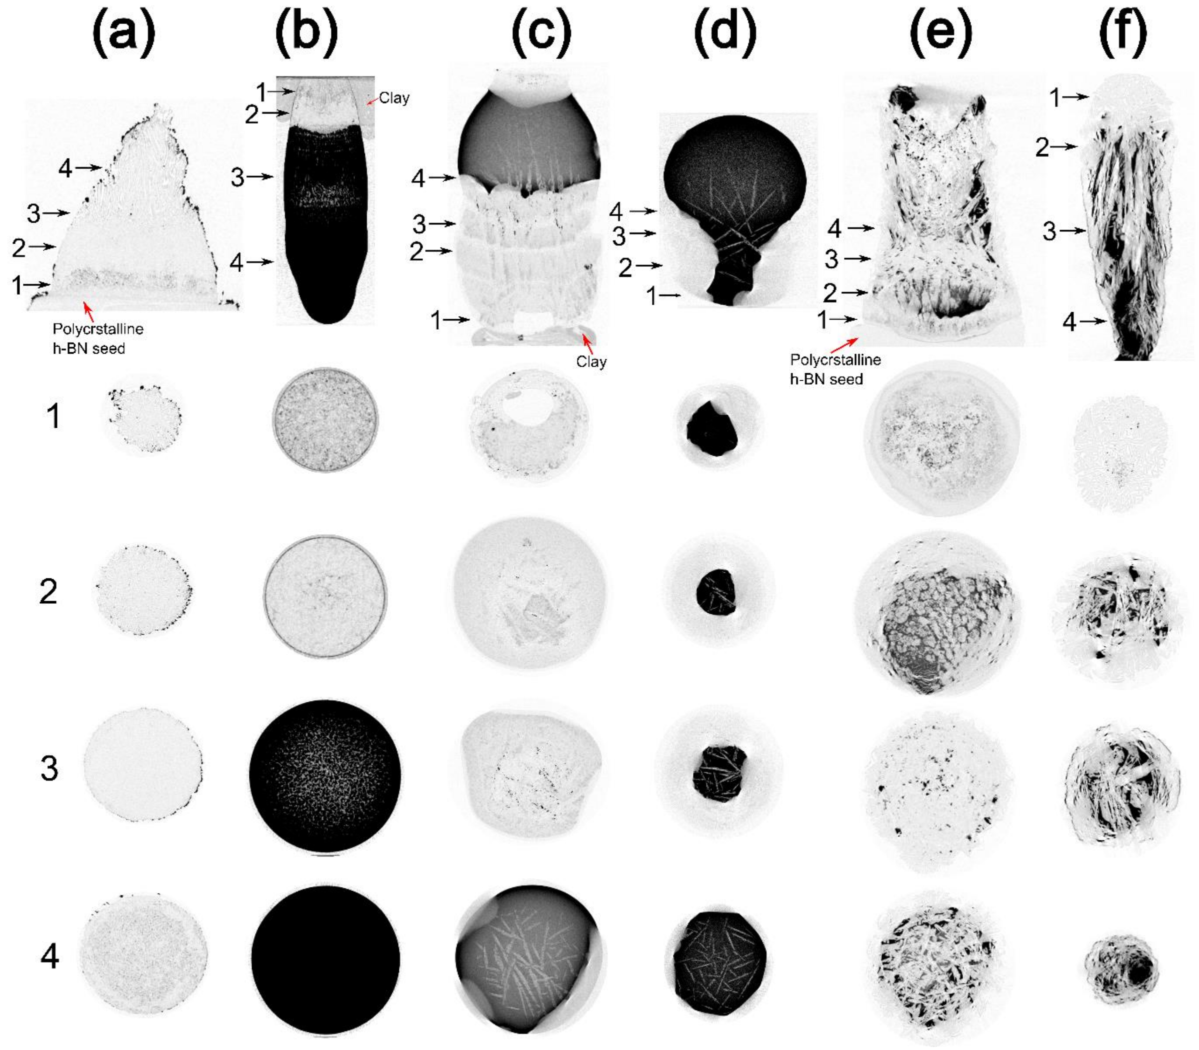


**Figure S2:** MicroCT data for the samples shown in Fig. S1, presented with the same format as Fig. 3 in the main text.

## 2. <u>Additional SEM/EDS data</u>

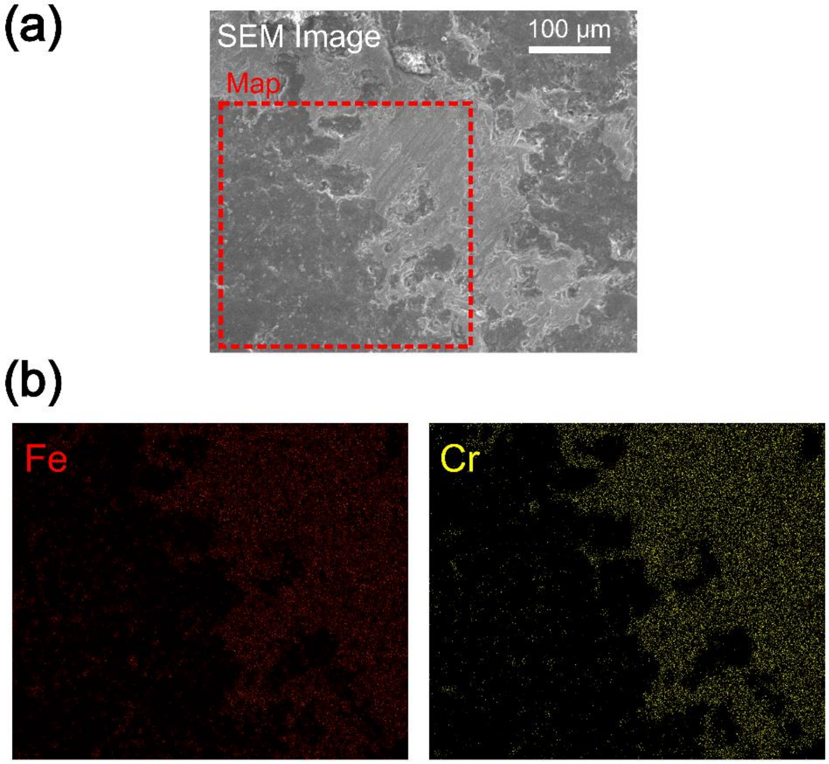


**Figure S3: (a)** Back-scattered electron SEM image of the sample shown in Fig. 4. **(b)** EDS map for Fe and Cr collected within the area surround by the dashed red line in **(a)**

## 3. X-ray diffraction data

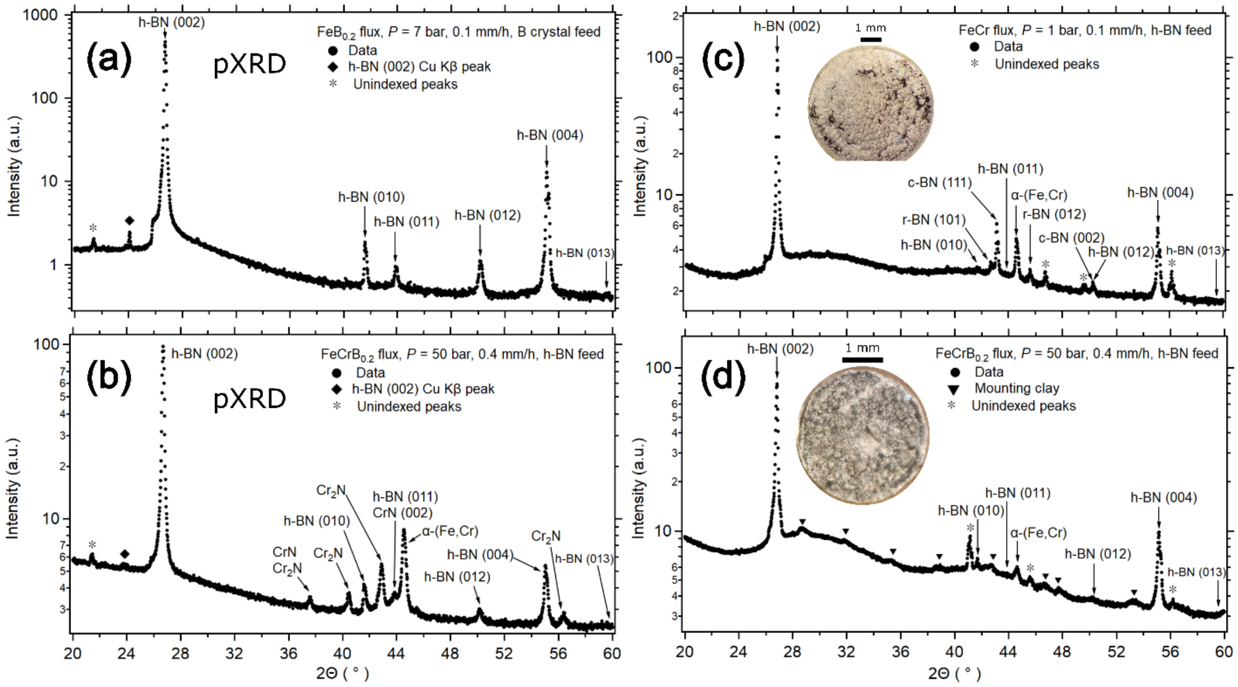


**Figure S4:** X-ray diffraction data on various samples grown by TSFZ. Note the log scale on the *y*-axis. **a)** PXRD data collected on a crushed section of the sample shown in Fig. S1d. **(b)** Data collected on a crushed section of the sample shown in Fig. 2b in the main text. **(c)** Data collected on the cut and polished sample shown in Fig. 4a. **(d)** Data collected on the cut and polished surface shown in the inset of Fig. 5c. The black triangles correspond to peaks from clay used to mount the sample in the diffractometer.

Figure S4 shows diffraction patterns collected on two samples grown by TSFZ with different fluxes and at different pressures. The data in Fig. S2a is from a powdered section of a low-pressure grown sample (Fig. S1d) which microCT data (Fig. S2d) showed to be flux free following aqua regia treatment. The data in Fig. S2b is from a powdered section of a high-pressure grown sample which microCT data showed contained flux inclusions encapsulated by h-BN (Fig. 2b). For the data in Fig. S2a all of the peaks can be indexed to h-BN (note that the (013) peak is expected to have very weak intensity) besides a weak peak at low-2Θ. As expected for a layered structure, there is strong preferred orientation for (00*L*) type peaks, boosting the relative intensity of these peaks considerably. The step like feature near the h-BN (002) peak is an instrumental artifact from the upstream Ni filter which is accentuated by the log scaling. Due to the strong intensity of the h-BN (002) peak the remnant Cu-$K_\beta$ radiation ($\lambda_{K\beta}$ = 1.392234 Å) produces a corresponding peak at 2Θ = 24.1° (black diamond). The data in Fig. S2b also shows peaks which can be indexed to h-BN, however there are more additional peaks. Consistent with the presence of trapped flux we see α-(Fe,Cr), as well as $Cr_2N$ and trace CrN (also observed in volatilized material). The small peak at 2Θ = 21.4° in Fig. S2a,b remains unidentified. However, it occurs with similar intensity in both samples and is therefore unlikely to be related to the flux since the proportion of trapped flux is very different.

The data presented in Fig. S2c,d shows diffraction patterns collected on two cut and polished samples (not powderized). These patterns largely show only (00*L*)-type h-BN peaks, with other peaks either absent or greatly reduced in intensity (e.g. the (010), which is expected to have 16% of the intensity of the (002) but is barely resolvable here). This indicates that the circular grains visible in the optical images and microCT data are largely (00*L*) oriented. Interestingly, in Fig. S2c we observe clear peaks which can be indexed by the cubic polymorph of BN (c-BN) and significantly smaller peaks which may be due to the rhombohedral polymorph (r-BN). The presence of other polymorphs was only observed in this sample. Lastly, we note that some of the unindexed peaks in these plots may actually be matched to a subset of $Cr_2N$ peak locations; however, the lack of powder averaging obscures the other $Cr_2N$ peaks, preventing a definitive identification.

## 4. Magnetomery data

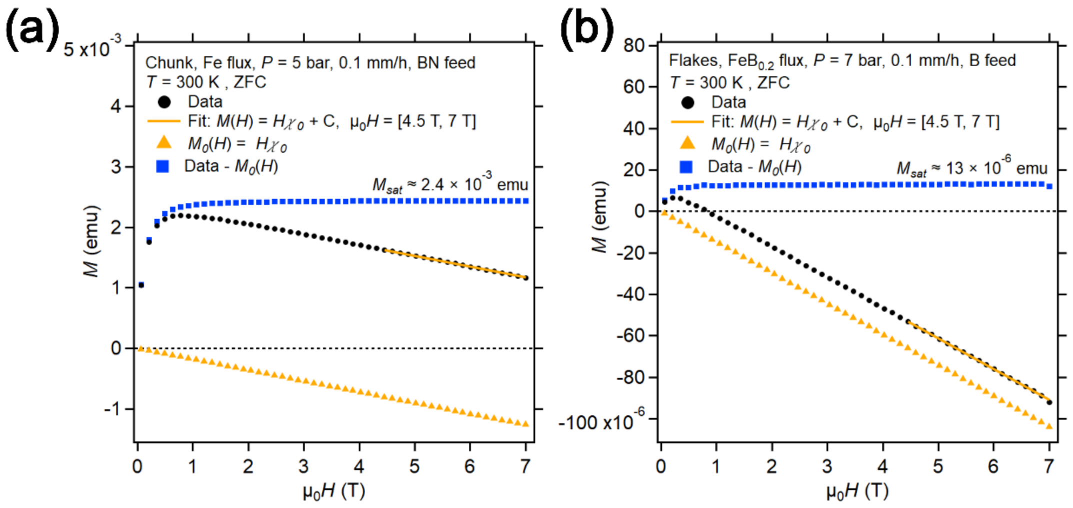


**Figure S5:** Unnormalized magnetization data collected on two different samples grown from Fe fluxes. **(a)** Data collected on a more three-dimensional "chunk" sample extracted from Stage 2 of the sample shown in Fig. 2a (red boxed area) following soaking in aqua regia and washing with ethanol. The sample mass was 2.8 mg. **(b)** Data collected on a collection of flake-like samples (see Fig. S6) extracted from the growth shown in Fig. S2d following soaking with aqua regia and washing with ethanol. The sample mass was 1.7 mg.

## 5. <u>Characterization of flake samples</u>

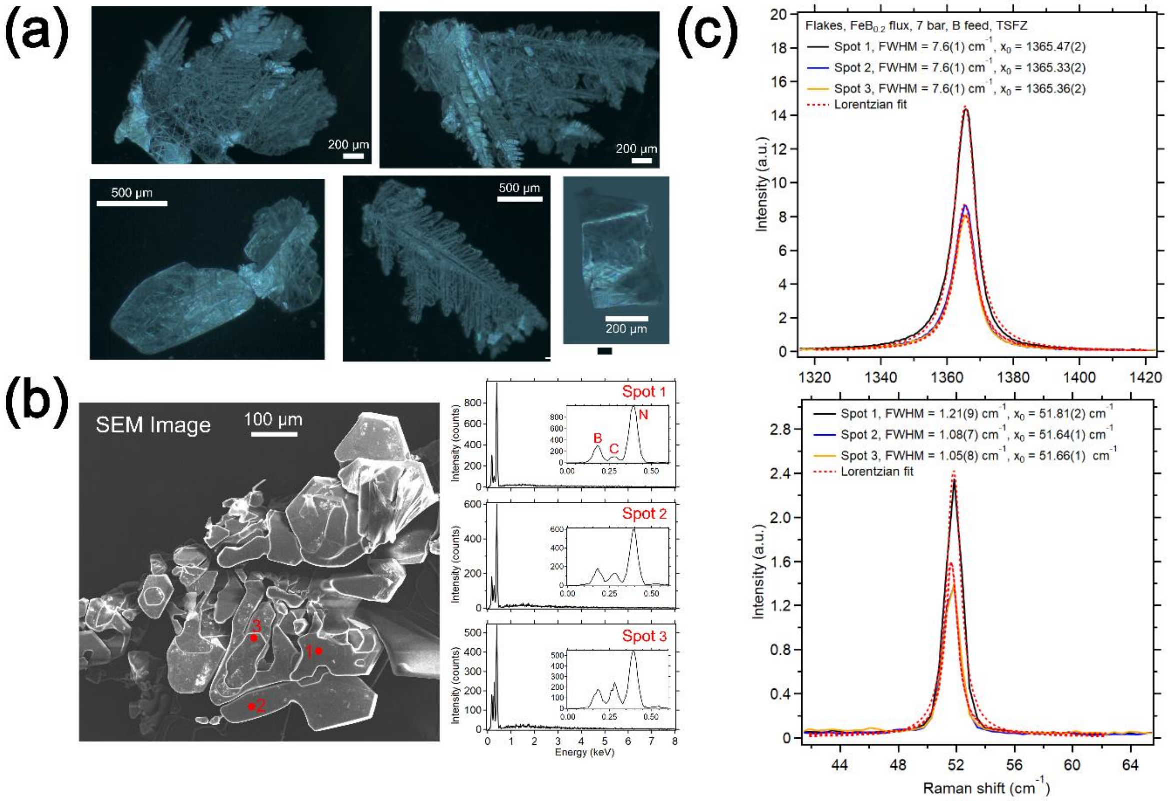


**Figure S6:** **(a)** Optical microscopy images of flake samples extracted from the interior of the sample shown in Fig. S1d following soaking in aqua regia and washing with ethanol. **(b)** SEM back-scattered electron image and EDS spot scans for a selected flake. **(c)** Raman data collected on a selected flake (with no cutting or polishing) showing sharp $E_{2g}$ modes. For the higher-energy (intralayer) mode the average FWHM is 7.6(2) $cm^{-1}$ and the average peak position is $x_0$ = 1365.39(3) $cm^{-1}$. For the lower-energy (interlayer) mode the average FWHM is 1.1(1) $cm^{-1}$ and the average peak position is $x_0$ = 51.70(2) $cm^{-1}$.

## 6. Additional Raman data

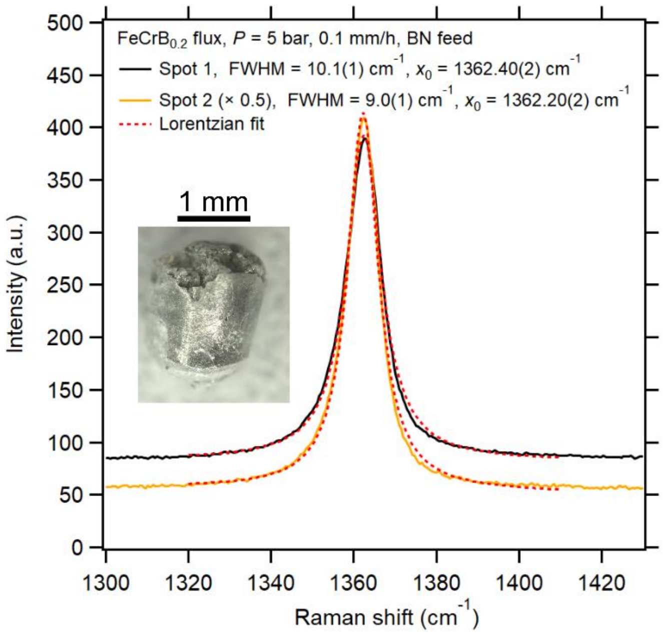


**Figure S7:** Raman data collected on Stage 2 of the sample shown in Fig. 2c in the main text, following soaking in aqua regia and washing with ethanol. No cutting or polishing was done prior to measurement. This measurement used a different spectrometer than the other reported data and the slight decrease of the peak position relative to other data sets (1362 $cm^{-1}$ versus 1365 $cm^{-1}$) is due to differences in calibration. The energy range of the lower-energy interlayer mode was not accessible in this measurement.

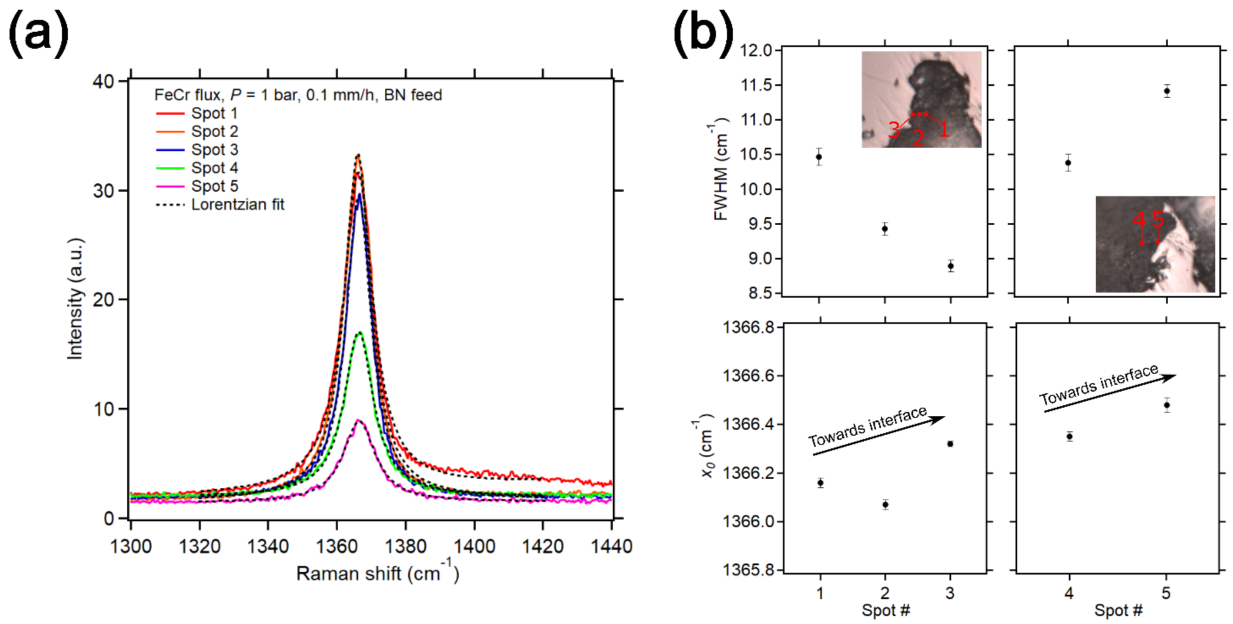


**Figure S8:** **(a)** Raman spectra for the h-BN intralayer mode collected sample shown in Fig. 4a. The growth parameters for this sample were: FeCr flux, $P = 1$ bar, 0.1 mm/h, h-BN feed, TSFZ, $\varphi = 0°$, $D_U = D_L = 6$ mm. Raman spectra were collected at various points in h-BN grains corresponding to different distances from the h-BN/flux interface. **(b)** Plots of the mode FWHM and position ($x_0$) as a function of distance to the h-BN/flux interface. No clear dependence on distance to the interface is observed for either parameter.
